# Supplementary material for: Tackling Shortcut Learning in Deep Neural Networks: An Iterative Approach with Interpretable Models
Source: arXiv:2302.10289 source file (2023-07-07)
Supplement: Supplementary file 1 [file completeness_v1.tex]

Let $f^0(x)=h^0(\Phi(\boldsymbol{x})$ is the initial Blackbox as per~\cref{sec:method}. The Concept completeness paper~\cite{yeh2019concept} assumes $\Phi(\boldsymbol{x}) \in \mathbb{R}^l$ (\st $l=T.d$) to be a concatanation of $[\phi(\boldsymbol{x}_1), \phi(\boldsymbol{x}_2), \dots, \phi(\boldsymbol{x}_T)]$ \st $\phi(\boldsymbol{x}) \in \mathbb{R}^d$. Recall we utilize $t$ to learn the concepts $\mathcal{C}$ with $N_c$ being the total number of concepts per image. So the parameters of $t$, represented by $\omega_1, \omega_2, \dots \omega_{N_c}$ \st $\omega_i \in \mathbb{R}^d$ represent linear direction in the embedding space $\phi(.) \in \mathbb{R}^d$. Next, we compute the concept product $v_c(\boldsymbol{x}_t)(<\phi(\boldsymbol{x}_t), \omega_j>)_{j=1}^{N_c}$, denoting the similarity between the image embedding and linear direction of $j^{th}$ concept. Finally, we normalize $v_c(.)$ to obtain the concept score as 
$v_v(\boldsymbol{x}) = \big(\frac{v_c(\boldsymbol{x_t})}{||v_c(\boldsymbol{x}_t)||_2}\big)_{t=1}^T \in \mathbb{R}^{T.{N_c}}$.

Next for a Blackbox $f^0(x)=h^0(\Phi(\boldsymbol{x})$, set of concepts $c_1, c_2, \dots c_{N_c}$ and their linear direction  $\omega_1, \omega_2, \dots \omega_{N_c}$ in the embedding space and, we compute the completeness score as:

\begin{align}
\eta_{f^0} = \frac{\text{sup}_\Gamma \mathbb{P}_{\boldsymbol{x}, y \sim V}
[y = \operatorname*{arg\,max}_{y'}h^0_{y'}(\Gamma(v_c(\boldsymbol{x})))] - a_r}{
\mathbb{P}_{\boldsymbol{x}, y \sim V}
[y = \operatorname*{arg\,max}_{y'}f^0_{y'}(\boldsymbol{x})] - a_r
},
\end{align}

where $V$ is the validation set and $\Gamma : \mathbb{R}^{T.m} \rightarrow \mathbb{R}^l$, projection from the concept score to the embedding space$\Phi$. For CUB-200 and Awa2 we estimate $\mathbb{P}_{\boldsymbol{x}, y \sim V}
[y = \operatorname*{arg\,max}_{y'}h^0_{y'}(\Gamma(v_c(\boldsymbol{x})))]$ as the best accuracy using the given concepts and $a_r$ is the random accuracy. For HAM10000, we estimate the same as the best AUROC. Completeness score indicates the consistency between the prediction based just on concepts and the given Blackbox$f^0$. If the identified concepts are sufficiently rich, label prediction will be similar to the Blackbox, resulting in higher completeness scores for the concept set. In all our experiments, $\Gamma$ is a two-layer feedforward neural network with 1000 neurons.
