# Supplementary material for: Tackling Shortcut Learning in Deep Neural Networks: An Iterative Approach with Interpretable Models
Source: arXiv:2302.10289 source file (2023-07-07)
Supplement: Supplementary file 2 [file concept_learning.tex]

% As discussed in~\cref{sec:method}, $f^0: \mathcal{X} \rightarrow \mathcal{Y}$ is a pre-trained Blackbox. Also, $\displaystyle f^0(.) =  h^0 \circ \Phi(.)$. Here, $ \Phi: \mathcal{X} \rightarrow R^l $ is the image embeddings, transforming the input images to an intermediate representation and $ h^0: R^l \rightarrow \mathcal{Y}$ is the classifier, classifying the output $\mathcal{Y}$ using the embeddings, $\Phi$. Our approach is applicable for both datasets with and without human-interpretable concept annotations. For datasets with the concept annotation $\mathcal{C} \in \mathbb{R}^{N_c}$ ($N_c$ being the number of concepts per image $\mathcal{X}$), we learn $t: R^l \rightarrow\mathcal{C}$ to classify the concepts using the embeddings. Per this definition, $t$ outputs a scalar value $c$ representing a single concept for each input image. 
% We adopt the concept learning strategy in PosthocCBM (PCBM)~\cite{yuksekgonul2022post} for datasets without concept annotation. 
% Specifically, we leverage a set of image embeddings with the concept being present and absent. Next, we learn a linear SVM ($t$) to construct the concept activation matrix~\cite{kim2017interpretability} as $\boldsymbol{Q} \in\mathbb{R}^{N_c \times l}$. 
% Finally we estimate the concept value as $c = \frac{<\Phi(x), q^i>}{||q_i||_2^2}$ $ \in \mathbb{R}$ utilizing each row $\boldsymbol{q^i}$ of $\boldsymbol{Q}$. Thus, the complete tuple of $j^{th}$ sample is $\{x_j, y_j, c_j\}$, denoting the image, label, and learned concept vector, respectively.
