# Supplementary material for: Tackling Shortcut Learning in Deep Neural Networks: An Iterative Approach with Interpretable Models
Source: arXiv:2302.10289 source file (2023-07-07)
Supplement: Supplementary file 3 [file algo_v1.tex]

% \begin{algorithm}[h]
%    \caption{\emph{Route, interpret} and \emph{Repeat} algorithm to generate FOL explanations locally.}
%    \label{algo: train}
% \begin{algorithmic}[1]
%    \STATE {\bfseries Input:} Complete tuple: \{$x_j$, $y_j$, $c_j$\}$_{j=1}^n$; initial blackbox $f^0 = h^0(\Phi(.))$; K as the total iterations; Coverages $\tau_1, \dots ,\tau_k$.
%    \STATE {\bfseries Output:} Sparse mixture of experts and their selectors $\{g^k, \pi^k\}_{k=1}^K$ and the final residual $f^K = h^K(\Phi(.))$
%    \STATE Fix $\Phi$.
%    \FOR{\texttt{$k=1 \dots K $}}
%        \STATE  Fix $\pi^1 \dots \pi^{k-1}$.
%        \STATE Swap $x_i$ and $x_{i+1}$.
%        \STATE Minimize $\mathcal{L}^k$ using equation \ref{equ:final_loss_g} to learn $\pi^k$ and $g^k$.
%        \STATE Calculate $r^k = f^{k-1}(.) - g^k(.)$
%        \STATE Minimize equation \ref{equ: residual} to learn $f^k(.)$, the new blackbox for the next iteration $k+1$.
%        \ENDFOR
%         \FOR{\texttt{$k=1 \dots K $}}
%             \FOR{sample $j$ in \texttt{test-set}}
%                 \REPEAT
%                     \STATE Initialize \texttt{sub\_select\_concept} = $True$
%                     \STATE Initialize the \texttt{percentile\_threshold} = $99$.
%                     \STATE Retrieve the predicted class label of sample $j$ from the expert $k$ as: $\hat{y}_j = g^k(c_j)$
%                     \STATE Create a mask vector $m_j$. $m_j[i] = 1$ if 
%                     $\Tilde{\alpha}[\hat{y}_j][i] \geq$ percentile$(\Tilde{\alpha}[\hat{y}_j]$, \texttt{percentile\_threshold}$)$ and $0$ otherwise. Specifically, the $i^{th}$ entry in $m_j$ is one if the $i^{th}$ value of the attention score $\Tilde{\alpha}[\hat{y}_j]$ is greater than (\texttt{percentile\_attention})$^{th}$ percentile. 
%                     \STATE Subselect the concept vector as $\Tilde{c}_j$ as: $\Tilde{c}_j = c_j\odot m_j$
%                     \IF{$g^k(\Tilde{c}_j) \neq \hat{y}_j$}
%                         \STATE \texttt{percentile\_threshold} = \texttt{percentile\_threshold} - 1
%                         \STATE \texttt{sub\_select\_concept} = $false$
%                     \ENDIF
%                 \UNTIL \texttt{sub\_select\_concept} is $True$
%                 \STATE Using the subselected concept vector $\Tilde{c_j}$, construct the FOL expression of the $j^{th}$ sample as suggested by~\cite{barbiero2022entropy}.
%             \ENDFOR
%     \ENDFOR
% \end{algorithmic}
% \end{algorithm}

% \cref{algo: train} explains the overall training procedure of our method.~\cref{fig:architecture} displays the architecture of our model in iteration $k$.


% % \begin{algorithm}
% % 	\caption{Training the MoIE to generate FOL explanations locally.} 
% % 	\label{algo: train}
% % 	\hspace*{\algorithmicindent} \textbf{Input:}  
% %         {
% %             Training set: \{$\mathcal{X}$, $\mathcal{Y}$, $\mathcal{S}$\}; trained blackbox $f^0 = h^0(\phi(.))$ using supervision of $\mathcal{Y}$; K as the \# iterations; Coverages $\tau_1, \dots ,\tau_k$
% %         } \\
% %         \hspace*{\algorithmicindent} \textbf{Output:}  
% %         {
% %             Sparse mixture of experts and their selectors $\{g^k, \pi^k\}_{k=1}^K$, 
% %         }
% % 	\begin{algorithmic}[1]
% %         \State Fix $\phi$.
% %         \State Train $t$ by minimizing BinaryCrossEnt($t(\phi(\boldsymbol{x})$, $\mathcal{S}$)
% %         \State Form a concept bank $\mathcal{C}$ with p concepts after discarding the concepts whose validation auroc (accuracy) $\leq$ 0.7 (70\%)
% %         \For{\texttt{iteration $k=1 \dots K $}}
% %             \State Fix $\pi^1 \dots \pi^{k-1}$.
% %             \State Minimize $\mathcal{L}^k$ using equation \ref{equ:final_loss_g} to learn $\pi^k$ and $g^k$.
% %             \State Calculate $r^k = f^{k-1}(.) - g^k(.)$
% %             \State Minimize equation \ref{equ: residual} to learn $f^k(.)$, the new blackbox for the next iteration $k+1$
% %         \EndFor
% %         \For{\texttt{experts $k=1 \dots K $}}
% %             \For{\texttt{each sample in the test-set}}
% %                 \State \label{12}Sort the concepts according to their attention scores from different experts in descending order.
% %                 \State Initialise FOL\_bucket as empty list.
% %                 \State Select one concept $\{c^i\}_{i=1}^p$ at a time from the sorted concept bank in step \ref{12} until 
% %                 \hspace*{\algorithmicindent} \quad $g(c^i$) = g($\boldsymbol{c}$) and add those concepts in the  FOL\_bucket.
% %                 \State Construct the FOL expression from FOL\_bucket using \cite{barbiero2022entropy}.
% %             \EndFor
% %         \EndFor
% % 	\end{algorithmic} 
% % \end{algorithm}
