# Supplementary material for: Tackling Shortcut Learning in Deep Neural Networks: An Iterative Approach with Interpretable Models
Source: arXiv:2302.10289 source file (2023-07-07)
Supplement: Supplementary file 4 [file loss_v1.tex]

% \begin{figure}[t]
% \centering
% \includegraphics[width=1\textwidth]
% {figures/Supp/Architecture.pdf}
% \caption{Architecture of MoIE. In an iteration $k$ during inference, the selector routes the samples through the interpretable expert $g^k$ if the probability $\pi^k \ge 0.5$. If $\pi^k < 0.5$, the selector routes the samples, through $f^k$, the Blackbox for iteration $k+1$. Note $f^k = h^k(\Phi(.)$ is an approximation of the residual $r^k = f^{k-1} - g^k$.  }
% \label{fig:architecture}
% \end{figure}

% In this section, we will discuss the loss function used in distilling the knowledge from the blackbox to the symbolic model. We remove the superscript $k$ for brevity. We adopted the optimization proposed in \cite{geifman2019selectivenet}.Specifically, we convert the constrained optimization problem in~\cref{equ: optimization_g} as 

% \begin{align}
% \label{equ:unconstrained_risk}
% &\mathcal{L}_s = \mathcal{R}(\pi, g) + \lambda_s \Psi(\tau - \zeta(\pi))\\ \nonumber
% &\Psi(a) = \text{max}(0, a)^2 ,
% \end{align}

% where $\tau$ is the target coverage and $\lambda_s$ is a hyperparameter (Lagrange multiplier). We define $\mathcal{R}(.)$ and $\mathcal{L}_{g, \pi}(.)$ in~\cref{equ: emp_risk} and~\cref{equ: g_k} respectively. $\ell$ in~\cref{equ: g_k} is defined as follows:

% \begin{align}
% \label{equ:ell}
% \ell\big(f, g \big) &= \ell_{distill}(f, g) + \lambda_{lens}\sum_{i=1}^r\mathcal{H}(\beta^i) ,
% \end{align}

% where $\lambda_{lens}$ and $\mathcal{H}(\beta^i)$ are the hyperparameters and entropy regularize, introduced in \cite{barbiero2022entropy} with $r$ being the total number of class labels. Specifically, $\beta^i$ is the categorical distribution of the weights corresponding to each concept.  To select only a few relevant concepts for each target class, higher values of $\lambda_{lens}$ will lead to a sparser configuration of $\beta$. $\ell$ is the knowledge distillation loss \cite{hinton2015distilling}, defined as 

% \begin{align}
% \label{equ:distill}
% \ell(f, g) = & (\alpha_{KD}* T_{KD}*T_{KD}) KL\big(\text{LogSoftmax}(g(.)/T_{KD}) , \text{Softmax}(f(.)/T_{KD})\big) + \\ \nonumber
% & (1 - \alpha_{KD}) CE\big(g(.), y\big),
% \end{align}

% where $T_{KD}$ is the temperature, CE is the Cross-Entropy loss, and $\alpha_{KD}$ is relative weighting controlling the supervision from the blackbox $f$ and the class label $y$.

% As discussed in \cite{geifman2019selectivenet}, we also define an auxiliary interpretable model using the same prediction task assigned to $g$ using the following loss function


% \begin{align}
% \label{equ:aux}
% \mathcal{L}_{aux} = \frac{1}{m}\sum_{j=1}^m\ell_{distill}(f(\boldsymbol{x_j}), g(\boldsymbol{c_j})) + \lambda_{lens}\sum_{i=1}^r\mathcal{H}(\beta^i),
% \end{align}
% which is agnostic of any coverage. $\mathcal{L}_{aux}$ is necessary for optimization as the symbolic model will focus on the target coverage $\tau$ before learning any relevant features, overfitting to the wrong subset of the training set. The final loss function to optimize by g in each iteration is as follows:

% \begin{align}
% \label{equ:final_loss_g}
% \mathcal{L} = \alpha \mathcal{L_s} + (1 - \alpha)\mathcal{L}_{aux},
% \end{align}

% where $\alpha$ is the can be tuned as a hyperparameter. Following \cite{geifman2019selectivenet}, we also use $\alpha=0.5$ in all of our experiments.
